# Supplementary material for: Efficient Model Learning and Adaptive Tracking Control of Magnetic Micro-Robots for Non-Contact Manipulation
Source: arXiv:2403.14414 source file (2024-03-21)
Supplement: Supplementary file 1 [file appendix.tex]

The  Lyapunov stability of the system with the control law \ref{eq: optimal} and updating law \ref{eq: online update} is analyzed as follows. Since $\bm u = \bm 0$ is a potential solution of the optimization problem, for the true optimal $\bm u$, we have 
\begin{equation}
    \frac{1}{2}\| \dot{\bm{x}}^d_u - \hat{\bm{g}}_u(s_r)\bm{u}\|^2 + \frac{\lambda}{2} \| \dot{\bm{x}}^d_r - \hat{\bm{g}}_r(s_r)\bm{u}\|^2 \leq \frac{1}{2}\| \dot{\bm{x}}^d_u\| + \frac{1}{2}\|\dot{\bm{x}}^d_r\|
\end{equation}
then expand the inequality
\begin{equation}
    -{(\hat{\bm{x}}^d_u)}^\intercal \hat{\bm{g}}_u(s_r)\bm{u} -{(\hat{\bm{x}}^d_r)}^\intercal \hat{\bm{g}}_r(s_r)\bm{u} + 
\end{equation}
